# Supplementary material for: A Non-linear Differentiable Model for Stormwater-based Irrigation of a Green Roof in Toronto
Source: arXiv:2110.13669 source file (2021-10-26)
Supplement: Supplementary file 1 [file Appendix.tex]

\section{Analysis of Value Functions}
The focus of this section is to prove Theorem \ref{lscremark}, which requires several intermediary results as depicted in Fig. \ref{illustration_of_theory}.
\begin{theorem}[Properties of $V_{t}^\theta$]\label{lscremark}
Assume Assumption \ref{measselect}. For all $t \in \mathbb{T}_N$, $V_{t}^\theta$ is lower semi-continuous (lsc) and bounded. For all $t \in  \mathbb{T}$, there is a Borel-measurable function $\mu_{t}^\theta : S \rightarrow A$ such that \eqref{existinf} holds. 
\end{theorem}
\begin{proof} By induction. For brevity, denote $\mathcal{S} := S \times A \times \mathbb{R}^d$. $V_N^\theta = c_N$ is lsc and bounded by Assumption \ref{measselect}. Now, suppose (the induction hypothesis) that for some $t \in \mathbb{T}$, $V_{t+1}^\theta$ is lsc and bounded. The key step is to show that $\psi_t^\theta$ \eqref{mypsi} is lsc and bounded.\footnote{If $\psi_t^\theta$ \eqref{mypsi} is lsc and bounded, then $v_{t+1}^\theta := c_t + \psi_t^\theta$ is lsc and bounded because the sum of two lsc and bounded functions is lsc and bounded. Since $v_{t+1}^\theta$ is bounded, $V_{t}^\theta$ is bounded \eqref{10b}. The remaining desired conclusions follow from a known result, which we will describe. Since $v_{t+1}^\theta : S \times A \rightarrow \mathbb{R}$ is lsc, $A$ is compact, and $V_{t}^\theta(x) := \inf_{u \in A} v_{t+1}^\theta(x,u)$, it holds that $V_{t}^\theta$ is lsc, and there is a Borel-measurable function $\mu_t^\theta : S \rightarrow A$ such that $V_{t}^\theta(x) = v_{t+1}^\theta(x,\mu_{t}^\theta(x))$ for all $x \in S$
by \cite[Prop. 7.33, p. 153]{bertsekas2004stochastic}. In summary, by assuming that $V_{t+1}^\theta$ is lsc and bounded, we will show that $\psi_t^\theta$ is lsc and bounded. The latter result will guarantee that $V_{t}^\theta$ is lsc and bounded \emph{and} the existence of a Borel-measurable function $\mu_t^\theta$ that satisfies \eqref{existinf}. This logic repeats backwards in time to complete the proof.} Boundedness of $\psi_t^\theta$ follows from boundedness of $V_{t+1}^\theta$. For showing boundedness, note that the function $\phi_t : \mathcal{S} \rightarrow \mathbb{R}$
\begin{equation}\label{myphi}
   \phi_t(x,u,w) := e^{\frac{-\theta}{2}V_{t+1}^\theta(f_t(x,u,w))}
\end{equation}
is non-negative and bounded. (We drop the superscript $\theta$ on the left-hand-side for brevity.) Also, for any $(x,u) \in S \times A$, the function $\phi_t(x,u,\cdot) : \mathbb{R}^d \rightarrow \mathbb{R}$ is Borel-measurable because it is a composition of Borel-measurable functions, and $p_t(\mathrm{d}w|x,u)$ is a probability measure on $(\mathbb{R}^d, \mathcal{B}_{\mathbb{R}^d})$. The above properties ensure that the (Lebesgue) integral
\begin{equation}\label{myphitprime}
    \phi_t'(x,u) := \textstyle \int_{\mathbb{R}^d } \phi_t(x,u,w) \; p_t(\mathrm{d}w|x,u)
\end{equation}
exists and is finite for all $(x,u) \in S \times A$. 

To complete the proof, we will show that $\psi_t^\theta$ \eqref{mypsi} is lsc. Since $f_t$ is continuous by Assumption \ref{measselect}, $V_{t+1}^\theta$ is lsc by the induction hypothesis, and $\frac{-\theta}{2} > 0$, the function $g_t : \mathcal{S} \rightarrow \mathbb{R}$
\begin{equation}\label{Myg}
 \textstyle   g_t(x,u,w) := \frac{-\theta}{2}V_{t+1}^\theta(f_t(x,u,w))
\end{equation}
is lsc.\footnote{Let $\{(x^i,u^i,w^i)\}_{i=1}^\infty$ be a sequence in $\mathcal{S}$ converging to $(x,u,w) \in \mathcal{S}$. To show that $V_{t+1}^\theta \circ f_t$ is lsc, we need to prove that
\begin{equation}
    \liminf_{i \rightarrow \infty} V_{t+1}^\theta(f_t(x^i,u^i,w^i)) \geq V_{t+1}^\theta(f_t(x,u,w))
\end{equation}
\cite[Lemma 7.13, p. 146]{bertsekas2004stochastic}. Since $\{(x^i,u^i,w^i)\}_{i=1}^\infty$ converges to $(x,u,w)$ and $f_t$ is continuous, $\{f_t(x^i,u^i,w^i)\}_{i=1}^\infty$ converges to $f_t(x,u,w)$. Since the latter is a converging sequence in $S$ and $V_{t+1}^\theta : S \rightarrow \mathbb{R}$ is lsc, we have
\begin{equation}\label{466}
    \liminf_{i \rightarrow \infty} V_{t+1}^\theta(f_t(x^i,u^i,w^i)) \geq V_{t+1}^\theta(f_t(x,u,w)),
\end{equation}
which proves that the composition $V_{t+1}^\theta \circ f_t$ is lsc. Since $V_{t+1}^\theta \circ f_t$ is lsc and $\frac{-\theta}{2} > 0$, $g_t := \frac{-\theta}{2}V_{t+1}^\theta \circ f_t$ is lsc because multiplying \eqref{466} by a positive constant preserves the direction of the inequality.} The next step is to show that $\phi_t$ \eqref{myphi}
is lsc. For this, we use Proposition \ref{prop1}, which we will prove after completing the current derivation.
\begin{proposition}[Comp. of con't, inc. and lsc]\label{prop1}
Let $\mathcal{M}$ be a metric space. Assume that $\mathcal{Y}_i := (a_i,b_i) \subseteq \mathbb{R}$ is non-empty for $i = 1,2$. Suppose that $\kappa_1 : \mathcal{Y}_1 \rightarrow \mathcal{Y}_2$ is continuous and increasing, and $\kappa_2 : \mathcal{M} \rightarrow \mathcal{Y}_1$ is lsc and bounded. (There are scalars $\underline{c}$ and $\overline{c}$ such that $[\underline{c}, \overline{c}] \subset \mathcal{Y}_1$ and $\underline{c} \leq \kappa_2(y) \leq \overline{c}$ for all $y \in \mathcal{M}$.) Then, $\kappa_1 \circ \kappa_2 : \mathcal{M} \rightarrow \mathcal{Y}_2$ is lsc.
\end{proposition}

Proposition \ref{prop1} specifies that the co-domain $\mathcal{Y}_i$ is an open subset of $\mathbb{R}$. We will use Proposition \ref{prop1} twice, and in the second case, $\mathcal{Y}_1 = (0,+\infty)$ and $\kappa_1 = \log$, which will ensure that the composition $\kappa_1 \circ \kappa_2$ is lsc and finite.

By Proposition \ref{prop1}, it holds that $\phi_t = \exp \circ g_t$ \eqref{myphi} is lsc because $\exp : \mathbb{R} \rightarrow (0,+\infty)$ is continuous and increasing and $g_t: \mathcal{S} \rightarrow \mathbb{R}$ \eqref{Myg} is lsc and bounded. In addition, $\phi_t$ is bounded as a consequence of $g_t$ being bounded.
%In Proposition \ref{prop1}, choose $\mathcal{M} = \mathcal{S}$, $\mathcal{Y}_1 = \mathbb{R}$, $\mathcal{Y}_2 = (0,+\infty)$, $\kappa_1 = \exp$, $\kappa_2 = g_t$, and $[\underline{c},\overline{c}] = [\frac{-\theta}{2}\underline{b},\frac{-\theta}{2}\overline{b}] \subset \mathcal{Y}_1$ so that $\phi_t = \kappa_1 \circ \kappa_2$.

It follows that $\phi_t'$ \eqref{myphitprime} is bounded and lsc. The latter property holds in particular because $\phi_t$ \eqref{myphi} is lsc and $p_t(\mathrm{d}w|x,u)$ is a continuous stochastic kernel (see Lemma \ref{phiprimeislsc}, to follow the proof of Prop. \ref{prop1}). We use Prop. \ref{prop1} to conclude that $\log \circ \; \phi_t' : S \times A \rightarrow \mathbb{R}$ is lsc. In Prop. \ref{prop1}, choose $\mathcal{M} = S \times A$, $\mathcal{Y}_1 = (0,+\infty)$, $\mathcal{Y}_2 = \mathbb{R}$, $\kappa_1 = \log$, $\kappa_2 = \phi_t'$, and $[\underline{c},\overline{c}] = [e^{\frac{-\theta}{2}\underline{b}},e^{\frac{-\theta}{2}\overline{b}}] \subset \mathcal{Y}_1$, where $\underline{b}$ is a lower bound and $\overline{b}$ is an upper bound for $V_{t+1}^\theta$. %so that $\kappa_1 \circ \kappa_2 = \log \circ \phi_t'$. , as $\log$ is continuous and increasing and $\phi_t'$ \eqref{myphitprime} is lsc and bounded
Finally, since $\log \circ \; \phi_t'$ is lsc and $\frac{-2}{\theta} > 0$, we conclude that $\psi_t := \frac{-2}{\theta} \log \circ \; \phi_t'$ is lsc.\end{proof}

Next, we will prove Proposition \ref{prop1}. A key aspect of the proof is the use of the bounds $\underline{c}$ and $\overline{c}$ to guarantee that a limit inferior is in the domain of $\kappa_1$. This and the continuity of $\kappa_1$ allow us to exchange the order of a limit and $\kappa_1$.

\begin{proof}[Prop. \ref{prop1}]
To show that $\kappa_1 \circ \kappa_2$ is lsc, we must show that
%\begin{equation}\label{my54}
   $ \liminf_{i \rightarrow \infty}  \kappa_1\big(\kappa_2(x^i)\big) \geq \kappa_1\big(\kappa_2(x)\big)$,
%\end{equation}
where $\{x^i\}_{i = 1}^\infty$ is a sequence in $\mathcal{M}$ converging to $x \in \mathcal{M}$. Since $\{x^i\}_{i = 1}^\infty$ converges to $x$ and $\kappa_2$ is lsc, it holds that
\begin{equation}\label{my717171}
  \lim_{i \rightarrow \infty} \inf_{k \geq i} \kappa_2(x^k) := \liminf_{i \rightarrow \infty} \kappa_2(x^i) \geq \kappa_2(x).
\end{equation}
%where we used the definition of the limit inferior to write the first expression. Note that $k \geq i$ is short-hand for $\{ k \in \mathbb{N} : k \geq i\}$. 
Since $\kappa_2$ is bounded below by $\underline{c}$ and above by $\overline{c}$, we have
\begin{equation}
\underline{c}   \leq \inf_{k \geq i} \kappa_2(x^k) \leq \inf_{k \geq i+1} \kappa_2(x^k) \leq \overline{c} \; \; \; \forall i \in \mathbb{N},
\end{equation}
which implies that
%\begin{equation}
  $\underline{c} \leq \lim_{i \rightarrow \infty} \inf_{k \geq i} \kappa_2(x^k) \leq \overline{c}$. 
%\end{equation}
Since $\{\inf_{k \geq i} \kappa_2(x^k)\}_{i=1}^\infty$ is a sequence in $[\underline{c}, \overline{c}]$ which converges to a point in $[\underline{c}, \overline{c}]$, $[\underline{c}, \overline{c}]$ is a non-empty subset of $\mathcal{Y}_1$, and $\kappa_1$ is continuous on $\mathcal{Y}_1$, we find that
\begin{equation}\label{my7474}
   \kappa_1 \Big( \lim_{i \rightarrow \infty} \inf_{k \geq i} \kappa_2(x^k) \Big) = \lim_{i \rightarrow \infty} \kappa_1 \Big( \inf_{k \geq i} \kappa_2(x^k) \Big).
\end{equation}
Since $\kappa_1$ is increasing and by \eqref{my717171}, we have
\begin{equation}\label{my757575}
 \kappa_1 \Big( \lim_{i \rightarrow \infty} \inf_{k \geq i} \kappa_2(x^k) \Big)  \geq \kappa_1 ( \kappa_2(x) ).
\end{equation}
%and by \eqref{my7474},
%\begin{equation}
%    \lim_{i \rightarrow \infty} \kappa_1 \Big( \inf_{k \geq i} \kappa_2(x^k) \Big) \geq \kappa_1 ( \kappa_2(x) ).
%\end{equation}
Moreover, since $\kappa_1$ is increasing, for any $i \in \mathbb{N}$, it holds that
\begin{equation}
   \forall k \geq i, \; \; \; \kappa_1(\kappa_2(x^k)) \geq \kappa_1 \Big( \inf_{k \geq i} \kappa_2(x^k) \Big).
\end{equation}
%Now, for any $i \in \mathbb{N}$,
%\begin{equation} 
 %   \forall k \geq i, \; \; \; \kappa_2(x^k) \geq \inf_{k \geq i} \kappa_2(x^k),
%\end{equation}
%and since $\kappa_1$ is increasing,
%\begin{equation}
 %  \forall k \geq i, \; \; \; \kappa_1(\kappa_2(x^k)) \geq \kappa_1 \Big( \inf_{k \geq i} \kappa_2(x^k) \Big).
%\end{equation}
Thus, $\kappa_1 \big( \inf_{k \geq i} \kappa_2(x^k) \big) \in \mathbb{R}$ is a lower bound for the set $\big\{ \kappa_1(\kappa_2(x^k)) : k \geq i\big\}$, which implies that
\begin{equation}\label{my7777}
    \inf_{k \geq i} \kappa_1(\kappa_2(x^k))  \geq \kappa_1 \Big( \inf_{k \geq i} \kappa_2(x^k) \Big).
\end{equation}
%which holds for all $i \in \mathbb{N}$.
%since the infimum is the greatest lower bound. Note that \eqref{my7777} holds for all %$i \in \mathbb{N}$. 
%Next, we discuss the limiting behavior of \eqref{my7777}. We have
%\begin{equation}
%  \lim_{i \rightarrow \infty}  \inf_{k \geq i} \kappa_1(\kappa_2(x^k)) := \liminf_{i \rightarrow \infty} \kappa_1(\kappa_2(x^i)),
%\end{equation}
%and by \eqref{my7474}, we have
 %  \begin{equation}
%    \lim_{i \rightarrow \infty} \kappa_1 \Big( \inf_{k \geq i} \kappa_2(x^k) \Big) = \kappa_1 \Big( \lim_{i \rightarrow \infty} \inf_{k \geq i} \kappa_2(x^k) \Big).
%\end{equation} 
By letting $i$ tend to infinity, it holds that
\begin{equation}
    \lim_{i \rightarrow \infty}  \inf_{k \geq i} \kappa_1(\kappa_2(x^k)) \geq \lim_{i \rightarrow \infty} \kappa_1 \Big( \inf_{k \geq i} \kappa_2(x^k) \Big),
\end{equation}
which is equivalent to
\begin{equation}
\liminf_{i \rightarrow \infty} \kappa_1(\kappa_2(x^i)) \geq \kappa_1 \Big( \lim_{i \rightarrow \infty} \inf_{k \geq i} \kappa_2(x^k) \Big)
\end{equation}
by \eqref{my7474}. Finally, by \eqref{my757575}, we derive the desired result,
\begin{equation}
\liminf_{i \rightarrow \infty} \kappa_1(\kappa_2(x^i)) \geq \kappa_1 ( \kappa_2(x) ).
\end{equation}\end{proof}

Subsequently, we will prove Lemma \ref{phiprimeislsc}, which we invoked in the proof of Theorem \ref{lscremark}.
\begin{lemma}[$\phi_t'$ is lsc and finite]\label{phiprimeislsc}
Recall that $\phi_t : S \times A \times \mathbb{R}^d \rightarrow (0,+\infty)$ is lsc and bounded \eqref{myphi}, and $p_t(\mathrm{d}w_t|x_t,u_t)$ is a continuous stochastic kernel on $\mathbb{R}^d$ given $S \times A$. It holds that $\phi_t' : S \times A \rightarrow (0,+\infty)$ \eqref{myphitprime} is lsc.
\end{lemma}
\begin{remark}[Regarding the proof of Lemma \ref{phiprimeislsc}]\label{myremark2}
The proof requires the following result, which is a special case of \cite[Prop. 7.31, p. 148]{bertsekas2004stochastic}. \emph{Let $\mathcal{X}$ and $\mathcal{Y}$ be separable metric spaces, and let $q(\mathrm{d}y|x)$ be a continuous stochastic kernel on $\mathcal{Y}$ given $\mathcal{X}$. Suppose that $g : \mathcal{X} \times \mathcal{Y} \rightarrow \mathbb{R}$ is lsc, and there are scalars $\underline{c}$ and $\overline{c}$ such that 
  $\underline{c} \leq g(x,y) \leq \overline{c}$ for all  $(x,y) \in \mathcal{X} \times \mathcal{Y}$.
It follows that the function $\lambda : \mathcal{X} \rightarrow \mathbb{R}$ defined by
\begin{equation}\label{functionlambda}
 \textstyle   \lambda(x) := \int_{\mathcal{Y}} g(x,y) \; q(\mathrm{d}y|x)
\end{equation}
is lsc.} Then, we choose $\mathcal{X} = S \times A$, $\mathcal{Y} = \mathbb{R}^d$, $g = \phi_t$, $\lambda = \phi_t'$, $\underline{c} = e^{\frac{-\theta}{2}\underline{b}}$, $\overline{c} = e^{\frac{-\theta}{2}\overline{b}}$, where $\underline{b}$ is a lower bound and $\overline{b}$ is an upper bound for $V_{t+1}^\theta$, and $q(\mathrm{d}y|x) = p_t(\mathrm{d}w|x,u)$. 

There are technicalities that will arise in the proof of Lemma \ref{phiprimeislsc} that deserve discussion. The proof requires the existence of a sequence of continuous functions that converges point-wise to a (given) lsc function. There are several similar results for this in the literature, e.g., see \cite[Theorem A6.6, pp. 390-391]{ash1972}, \cite[Lemma 7.14, pp. 147-148]{bertsekas2004stochastic}, and \cite[pp. 50-51]{dynkin}. To apply these existing results to our setting, a technical explanation is required, which is the purpose of the statement and proof of Lemma \ref{lscbounded}.
%These existing results may require further clarification to explain how they apply to our setting, which is our motivation for including Lemma \ref{lscbounded}. 
The (not necessarily unique) function sequence must have a common lower bound to apply the Monotone Convergence Theorem in a subsequent step, and Lemma \ref{lscbounded} specifies such a lower bound. Also, we will construct a sequence in a metric space whose limit exists and equals zero, and we will prove the existence and the value of this limit. Next, we will provide a proof for Lemma \ref{phiprimeislsc}, and a proof for Lemma \ref{lscbounded} will follow.
\end{remark}
\begin{proof}[Lemma \ref{phiprimeislsc}]
Recall that it suffices to prove the result that is stated in Remark \ref{myremark2}. For this, we will use three facts. First, note that $g : \mathcal{X} \times \mathcal{Y} \rightarrow \mathbb{R}$ being lsc and bounded ($\underline{c} \leq g \leq \overline{c}$), where $\mathcal{X} \times \mathcal{Y}$ is a metric space, implies that there is a sequence of continuous functions $g_m : \mathcal{X} \times \mathcal{Y} \rightarrow \mathbb{R}$ such that $\underline{c} \leq g_m \leq g_{m+1} \leq g \leq \overline{c}$ for all $m \in \mathbb{N}$, and $\{g_m\}_{m=1}^\infty$ converges to $g$ point-wise (Lemma \ref{lscbounded}).
%\begin{enumerate}
 %   \item $\underline{c} \leq g_m(x,y) \leq g_{m+1}(x,y) \leq g(x,y) \leq \overline{c}$ for all $(x,y) \in \mathcal{X} \times \mathcal{Y}$ and $m \in \mathbb{N}$, and
 %   \item $\lim_{m \rightarrow \infty} g_m(x,y) = g(x,y)$ for all $(x,y) \in \mathcal{X} \times \mathcal{Y}$.
%\end{enumerate}

The second fact is \cite[Prop. 7.30, p. 145]{bertsekas2004stochastic}, which ensures that the function $\lambda_m : \mathcal{X} \rightarrow \mathbb{R}$ defined by
\begin{equation}
  \textstyle   \lambda_m(x) := \int_{\mathcal{Y}}  g_m(x,y) \; q(\mathrm{d}y|x)
\end{equation}
is continuous for all $m \in \mathbb{N}$.\footnote{Continuity holds as a consequence of $\mathcal{X}$ and $\mathcal{Y}$ being separable metric spaces, $q(\mathrm{d}y|x)$ being a continuous stochastic kernel on $\mathcal{Y}$ given $\mathcal{X}$, and $g_m$ being bounded and continuous on $\mathcal{X} \times \mathcal{Y}$.}
%
%$\mathcal{X}$ and $\mathcal{Y}$ are separable metric spaces, $q(\mathrm{d}y|x)$ is a continuous stochastic kernel on $\mathcal{Y}$ given $\mathcal{X}$, $g_m : \mathcal{X} \times \mathcal{Y} \rightarrow \mathbb{R}$ is bounded and continuous for all $m \in \mathbb{N}$, and thus the function
%Now, if $\{x_n\}_{n=1}^\infty \subseteq \mathcal{X}$ converges to $x \in \mathcal{X}$, continuity of $\lambda_m$ implies that 
%Let $\rho : \mathcal{X} \times \mathcal{X} \rightarrow [0,+\infty)$ be the metric on $\mathcal{X}$, and let $\{x_n\}_{n=1}^\infty \subseteq \mathcal{X}$ be a sequence in $\mathcal{X}$ and $x \in \mathcal{X}$ such that the limit of $\{\rho(x_n,x)\}_{n = 1}^\infty$ equals 0. Since $\lambda_m$ is continuous for all $m \in \mathbb{N}$, we have
%\begin{equation}\label{my8888}
  %  \lim_{n \rightarrow \infty} \lambda_m(x_n) = \lambda_m(x). %\;\;\;\forall m \in \mathbb{N}.
%\end{equation}

The third fact is the Extended Monotone Convergence Theorem \cite[p. 47]{ash1972}, which allows us to conclude that
\begin{equation}\label{my8989}
   \lim_{m \rightarrow \infty} \underbrace{\textstyle  \int_{\mathcal{Y}} g_m(x,y) \; q(\mathrm{d}y|x)}_{\lambda_m(x)} = \underbrace{\textstyle \int_{\mathcal{Y}} g(x,y) \; q(\mathrm{d}y|x)}_{\lambda(x)}.
\end{equation}
For this, use a measure space $(\mathcal{Y},\mathcal{B}_{\mathcal{Y}}, q(\mathrm{d}y|x))$, which is parameterized by $x$. Define $h : \mathcal{Y} \rightarrow \mathbb{R}$ such that $h(y) = \underline{c}$ for all $y \in \mathcal{Y}$. The functions $g_m(x,\cdot): \mathcal{Y} \rightarrow \mathbb{R}$, $g(x,\cdot): \mathcal{Y} \rightarrow \mathbb{R}$, and $h : \mathcal{Y} \rightarrow \mathbb{R}$ are Borel-measurable. %relative to $\mathcal{B}_{\mathcal{Y}}$ and $\mathcal{B}_{\mathbb{R}}$. 
It holds that $g_m(x,\cdot) \geq h$ for all $m \in \mathbb{N}$, where $\int_{\mathcal{Y}} h(y) q(\mathrm{d}y|x) = \underline{c} > -\infty$, and $g_m(x,\cdot) \uparrow g(x,\cdot)$. Thus, $\int_{\mathcal{Y}} g_m(x,y)  q(\mathrm{d}y|x) \uparrow \int_{\mathcal{Y}} g(x,y)  q(\mathrm{d}y|x)$ by \cite[Thm. 1.6.7, p. 47]{ash1972}.
 
We will use the above facts to prove that $\lambda$ \eqref{functionlambda} is lsc by showing that
\begin{equation}\label{toshowfunctionlambda}
 \liminf_{n \rightarrow \infty} \underbrace{\textstyle \int_{\mathcal{Y}} g(x_n,y) \; q(\mathrm{d}y|x_n)}_{\lambda(x_n)} \geq \underbrace{\textstyle \int_{\mathcal{Y}} g(x,y) \; q(\mathrm{d}y|x)}_{\lambda(x)},
\end{equation}
where $\{x_n\}_{n =1}^\infty$ is a sequence in $\mathcal{X}$ converging to $x \in \mathcal{X}$. Since $g \geq g_m \geq \underline{c}$ for all $m \in \mathbb{N}$ and these functions are Borel-measurable, it follows that
\begin{equation}\label{my44}
    \underbrace{\textstyle \int_{\mathcal{Y}} g(x_n,y)\; q(\mathrm{d}y|x_n)}_{\lambda(x_n)} \geq \underbrace{\textstyle \int_{\mathcal{Y}} g_m(x_n,y) \; q(\mathrm{d}y|x_n)}_{\lambda_m(x_n)}
\end{equation}
for all $n \in \mathbb{N}$ and $m \in \mathbb{N}$. %by \cite[Theorem 1.5.9 (b), p. 41]{ash1972}. 
%In particular, use a measure space $(\mathcal{Y},\mathcal{B}_{\mathcal{Y}}, q(\mathrm{d}y|x_n))$, which is parameterized by $x_n$, and note that $g(x_n, \cdot) : \mathcal{Y} \rightarrow \mathbb{R}$ and $g_m(x_n, \cdot) : \mathcal{Y} \rightarrow \mathbb{R}$ for all $m \in \mathbb{N}$ are measurable relative to $\mathcal{B}_{\mathcal{Y}}$ and $\mathcal{B}_{\mathbb{R}}$. 
Since $\lambda_m$ is continuous for all $m \in \mathbb{N}$ and by \eqref{my44}, we have
\begin{equation}\label{my29}
     \liminf_{n \rightarrow \infty} \lambda(x_n) \geq \liminf_{n \rightarrow \infty} \lambda_m(x_n) = \lambda_m(x) \; \; \; \forall m \in \mathbb{N}.
\end{equation}
Finally, by using \eqref{my29} and \eqref{my8989}, we conclude that
\begin{equation}\begin{aligned}
    \liminf_{n \rightarrow \infty} \lambda(x_n) & \geq \lim_{m \rightarrow \infty} \lambda_m(x) = \lambda(x),
\end{aligned}\end{equation}
which shows \eqref{toshowfunctionlambda}. %and therefore proves that $\lambda$ is lsc.
\end{proof}
%
%In the following lemma, we show a useful property of lower semi-continuous functions. Similar results and proofs can be found in \cite[Theorem A6.6, pp. 390-391]{ash1972}, \cite[Lemma 7.14, pp. 147-148]{bertsekas2004stochastic}, and \cite[pp. 50-51]{dynkin}. Specifically, our proof shows why the limit of the sequence $\{\rho(x,y_m)\}_{m=1}^\infty$ exists, and the existence of this limit is required for the proof to hold.

Next, we prove Lemma \ref{lscbounded}, which we invoked previously.
\begin{lemma}[Existence of inc. seq. con't]\label{lscbounded}
Let $\mathcal{M}$ be a metric space, and let $h : \mathcal{M} \rightarrow \mathbb{R}$ be lsc and bounded. In particular, there are scalars $\underline{c}$ and $\overline{c}$ such that $\underline{c} \leq h(x) \leq \overline{c}$ for all $ x \in \mathcal{M}$. Then, there is a sequence of continuous functions $h_m : \mathcal{M} \rightarrow \mathbb{R}$ such that $\underline{c} \leq h_m \leq h_{m+1} \leq h \leq \overline{c}$ for all $m \in \mathbb{N}$, and $\{h_m\}_{m=1}^\infty$ converges point-wise to $h$.
%\begin{enumerate}
%    \item $\underline{c} \leq h_m \leq h_{m+1} \leq h \leq \overline{c}$ for all $x \in \mathcal{M}$ and $m \in \mathbb{N}$, and
 %   \item $\lim_{m \rightarrow \infty} h_m(x) = h(x)$ for all $x \in \mathcal{M}$.
%\end{enumerate}
\end{lemma}
\begin{proof}
We start by defining $h_m: \mathcal{M} \rightarrow \mathbb{R}^*$ in the typical way,
%For any $m \in \mathbb{N}$, define $h_m : \mathcal{M} \rightarrow \mathbb{R}^*$ as follows:
%\begin{equation}
 $   h_m(x) := \inf\{ h(y) + m \rho(x,y) : y \in \mathcal{M}\}$,
%\end{equation}
where $\rho : \mathcal{M} \times \mathcal{M} \rightarrow [0,+\infty)$ is the metric on $\mathcal{M}$ and $m \in \mathbb{N}$. $h_m$ is uniformly continuous on $\mathcal{M}$ (e.g., see \cite[p. 126]{bertsekas2004stochastic}). Since $h$ is bounded below by $\underline{c}$ and $\rho$ is bounded below by 0, it holds that $\underline{c} + 0 \leq  h(y) + m \rho(x,y) \leq h(y) + (m+1) \rho(x,y)$ for all $(x,y) \in \mathcal{M} \times \mathcal{M}$ and $m \in \mathbb{N}$, which implies that
%, and $0 \leq m \leq m+1$ for all $m \in \mathbb{N}$, 
%it follows that
%\begin{equation}
 %  \underline{c} + 0 \leq  h(y) + m \rho(x,y) \leq h(y) + (m+1) \rho(x,y)
%\end{equation}
%for all $(x,y) \in \mathcal{M} \times \mathcal{M}$ and $m \in \mathbb{N}$, which %implies that
\begin{equation}
    \underline{c} \leq h_m(x) \leq h_{m+1}(x) \; \; \; \forall x \in \mathcal{M}, \; \forall m \in \mathbb{N}.
\end{equation}
%For any $x \in \mathcal{M}$ and $m \in \mathbb{N}$, 
Since $\{ h(y) + m \rho(x,y) : y \in \mathcal{M}\}$ is a subset of $\mathbb{R}$ that is bounded below, $h_m(x)$ is finite.
%
%it holds that Recall that the infimum of a subset of $\mathbb{R}$ that is bounded below is finite. Therefore, for any $x \in \mathcal{M}$ and $m \in \mathbb{N}$, $h_m(x)$ is finite. Thus, for any $m \in \mathbb{N}$, we write $h_m : \mathcal{M} \rightarrow \mathbb{R}$. 
In addition,
%\begin{equation}
   $ h_m(x) \leq h(x) + m \rho(x,x) = h(x) \leq \overline{c}$ for all $x \in \mathcal{M}$ and $m \in \mathbb{N}$.
%\end{equation}

Now, let $x \in \mathcal{M}$. We have shown that $\{h_m(x)\}_{m=1}^\infty$ is an increasing sequence in $\mathbb{R}$ that is bounded above by $h(x) \in \mathbb{R}$. It follows that the limit of the sequence exists and
\begin{equation}\label{my99}
    \lim_{m \rightarrow \infty} h_m(x) \leq h(x).
\end{equation}
Next, we will show that \eqref{my99} holds with equality. Since the infimum $h_m(x)$ is finite, 
%For all $m \in \mathbb{N}$, $h_m(x) \in \mathbb{R}$, which implies that
for all $\epsilon > 0$, there is a point $y_{m} \in \mathcal{M}$ such that $h(y_m) + m \rho(x,y_m) \leq h_m(x) + \epsilon$, 
%\begin{equation}
%    \forall \epsilon > 0 \; \exists y_{m} \in \mathcal{M} \; \text{s.t. } h(y_m) + m \rho(x,y_m) \leq h_m(x) + \epsilon,
%\end{equation}
%by the definition of the infimum, 
where $y_m$ depends on $\epsilon$ and $x$. 

Now, let $\epsilon > 0$, and we will use this $\epsilon$ for all $m \in \mathbb{N}$.
%Let $\epsilon > 0$. 
Since $h_m(x) \in \mathbb{R}$, there is a point $y_m \in \mathcal{M}$ such that
\begin{equation}\label{my103}
    h(y_m) + m\rho(x,y_m) \leq h_m(x) + \epsilon.
\end{equation}
By continuing this process for all $m \in \mathbb{N}$, we obtain a sequence $\{y_m\}_{m=1}^\infty \subseteq \mathcal{M}$, where each $y_m$ satisfies \eqref{my103}.
%and we obtain a sequence 
%Since $h_2(x) \in \mathbb{R}$, there is a point $y_2 \in \mathcal{M}$ such that
%\begin{equation}
 %   h(y_2) + 2\rho(x,y_2) \leq h_2(x) + \epsilon.
%\end{equation}
%By continuing this process for all $m \in \mathbb{N}$, we obtain a sequence $\{y_m\}_{m=1}^\infty$ in $\mathcal{M}$ such that
%\begin{equation}\label{my103}
 %  h(y_m) + m \rho(x,y_m) \leq h_m(x) + \epsilon \;\;\; \forall m \in \mathbb{N}. 
%\end{equation}
%In addition, 
Since $\underline{c} \leq h(y_m)$ and $h_m(x) \leq h(x)$ for all $m \in \mathbb{N}$, it follows that
%\begin{equation}\begin{aligned}
%\underline{c} +  m \rho(x,y_m) \leq  h(y_m) + m \rho(x,y_m) \leq h_m(x) + \epsilon
%\end{aligned}\end{equation}
%for all $m \in \mathbb{N}$. By the previous statement and $h_m(x) \leq h(x)$ for all $m \in \mathbb{N}$, we find that
\begin{equation}
    \underline{c} +  m \rho(x,y_m) \leq  h_m(x) + \epsilon \leq h(x) + \epsilon \;\;\; \forall m \in \mathbb{N}.
\end{equation}
Since $\underline{c} \in \mathbb{R}$, $m > 0$ is finite, and $\rho$ is bounded below by 0, it holds that
\begin{equation}\label{my106}
    0 \leq \rho(x,y_m) \leq \frac{h(x) + \epsilon - \underline{c}}{m}\;\;\;\;\;\; \forall m \in \mathbb{N}.
\end{equation}
The inequality \eqref{my106} and $h(x)$ being finite imply that
\begin{equation}
    \liminf_{m \rightarrow \infty} \rho(x,y_m) = \limsup_{m \rightarrow \infty} \rho(x,y_m) = 0,
\end{equation}
which shows that the limit of $\{\rho(x,y_m)\}_{m=1}^\infty$ exists and equals zero.
%Therefore, the limit of $\{\rho(x,y_m)\}_{m=1}^\infty$ exists and
%\begin{equation}
%    \lim_{m \rightarrow \infty} \rho(x,y_m) = 0.
%\end{equation}
Since $h$ is lsc and $\{y_m\}_{m=1}^\infty \subseteq \mathcal{M}$ converges to $x \in \mathcal{M}$, we have that %the following inequality holds:
%\begin{equation}\label{my109}
    $h(x) \leq \liminf_{m \rightarrow \infty} h(y_m)$.
%\end{equation}
In addition, by using \eqref{my103} and $m \rho(x,y_m) \geq 0$, it holds that
%\begin{equation}
  %$h(y_m) \leq h(y_m) + m \rho(x,y_m) \leq h_m(x) + \epsilon$ for all $ m \in \mathbb{N}$,
   $h(y_m) \leq h_m(x) + \epsilon$ for all $ m \in \mathbb{N}$,
%\end{equation}
and therefore,
\begin{equation}
h(x) \leq \liminf_{m \rightarrow \infty}  h(y_m) \leq \liminf_{m \rightarrow \infty} h_m(x) + \epsilon.
\end{equation}
%Moreover, by \eqref{my109}, it holds that
%\begin{equation}
 %   h(x) \leq \liminf_{m \rightarrow \infty} h(y_m) \leq \liminf_{m \rightarrow \infty} h_m(x) + \epsilon.
%\end{equation}
Since the limit of $\{h_m(x)\}_{m=1}^\infty$ exists 
%, we have 
%\begin{equation}
 %       h(x) \leq \liminf_{m \rightarrow \infty} h(y_m) \leq \lim_{m \rightarrow \infty} h_m(x) + \epsilon,
%\end{equation}
and is less than $h(x)$ \eqref{my99}, it follows that
\begin{equation}
     h(x) \leq \lim_{m \rightarrow \infty} h_m(x) + \epsilon \leq h(x) + \epsilon.
\end{equation}
Since $h(x) \in \mathbb{R}$, we find that
%\begin{equation}
    $\big|-\hspace{-.5mm}h(x) + \lim_{m \rightarrow \infty} h_m(x)\big| \leq \epsilon$.
%\end{equation}
Finally, since the analysis holds for all $\epsilon > 0$ and $x \in \mathcal{M}$, we conclude that $\lim_{m \rightarrow \infty} h_m(x) = h(x)$ for all $x \in \mathcal{M}$.
%\begin{equation}
 %   \lim_{m \rightarrow \infty} h_m(x) = h(x) \;\;\; \forall x \in \mathcal{M}.
%\end{equation}
%For any $m \in \mathbb{N}$, to show that $h_m : \mathcal{M} \rightarrow \mathbb{R}$ is %continuous, by using a symmetry argument as in \cite[p. 126]{bertsekas2004stochastic}, %it holds that $h_m$ is uniformly continuous on $\mathcal{M}$.
%\begin{equation}
 %   |h_m(x) - h_m(y)| \leq m \rho(x,y) \;\;\; \forall (x,y) \in \mathcal{M} \times \mathcal{M}.
%\end{equation}
%Let $\epsilon > 0$, and choose $\delta := \frac{\epsilon}{m}$. If $(x,y) \in \mathcal{M} \times \mathcal{M}$ satisfies $\rho(x,y) < \delta$, then
%\begin{equation}
  %\textstyle   |h_m(x) - h_m(y)| \leq m \rho(x,y) < m \delta = m \frac{\epsilon}{m} = %\epsilon.
%\end{equation}
%We have shown that for all $\epsilon > 0$, there is a $\delta > 0$ such that $\rho(x,y) %< \delta$ and $(x,y) \in \mathcal{M} \times \mathcal{M}$ imply that $|h_m(x) - h_m(y)| < %\epsilon$. Therefore, $h_m$ is uniformly continuous on $\mathcal{M}$.
\end{proof}

We have completed our proofs of the building blocks that underlie Theorem \ref{lscremark} (Fig. \ref{illustration_of_theory}). Thus, we have ensured that the value functions $V_t^\theta$ satisfy key properties.
%
%The last two results are used to show the existence of a policy that is optimal for $V_\theta^*$ by invoking Assumption \ref{measselect}.
%
\section{Existence of an Optimal Risk-Averse Policy}
Here, we will prove a dynamic programming recursion for the risk-averse control problem (Lemma \ref{dynprogremark}). Then, we will use Lemma \ref{dynprogremark} and Theorem \ref{lscremark} to show that $V_{0}^\theta = V_{\theta}^*$ and the existence of an optimal risk-averse policy (Theorem \ref{optimality}). 

Define the random cost-to-go $Z_t$ for time $t \in \mathbb{T}_N$ as follows: for all $\omega = (x_0,u_0,\dots,x_{N-1},u_{N-1},x_N) \in \Omega$, % := (\mathbb{R}^n \times A)^N \times \mathbb{R}^n$,
\begin{equation}\label{myZt}
  \textstyle  Z_t(\omega) := \begin{cases} c_N(x_N) + \sum_{i=t}^{N-1} c_i(x_i,u_i) &  \text{if } t \in \mathbb{T} \\ c_N(x_N) & \text{if } t = N\end{cases}.
\end{equation}
Note that $Z_t(\omega) = c_t(x_t,u_t) + Z_{t+1}(\omega)$ for any $t \in \mathbb{T}$ and $\omega \in \Omega$ of the form specified above, and $Z_0 = Z$ \eqref{myZ}. While $Z_t$ is a random variable whose domain is $\Omega$, $Z_t$ does \emph{not} depend on the trajectory prior to time $t$, which is critical for deriving a dynamic programming recursion that is history-dependent only through the current state. For any $t \in \mathbb{T}_N$, $x \in S$, $\theta \in \Theta$, and $\pi \in \Pi$, we denote a conditional expectation of $e^{\frac{-\theta}{2} Z_t}$ by
%\begin{equation}\label{condexp}
  $ W_t^{\pi,\theta}(x) := E^\pi(e^{\frac{-\theta}{2} Z_t}| X_t = x )$.
%\end{equation}
%Note that the function $W_t^{\pi,\theta} : S \rightarrow \mathbb{R}^*$ is 
%Borel-measurable \cite[Thm. 6.3.3, p. 245]{ash1972}. %The following result provides a recursion for $W_t^{\pi,\theta}$.

\begin{lemma}[A DP recursion]\label{dynprogremark}
Let $\theta \in \Theta$ and $\pi = (\mu_0,\mu_1,\dots,\mu_{N-1}) \in \Pi$. Under Assumption \ref{measselect}, it holds that $W_t^{\pi,\theta}(x)\in (0,+\infty)$ for all $x \in S$, and
\begin{equation*}\begin{aligned}
& W_t^{\pi,\theta}(x) =\\
 &  \textstyle e^{\frac{-\theta}{2}c_t(x,\mu_t(x))}  \int_{\mathbb{R}^d} W_{t+1}^{\pi,\theta}(f_t(x,\mu_t(x),w)) \; p_t(\mathrm{d}w|x,\mu_t(x))
\end{aligned}\end{equation*}
for all $t \in \mathbb{T}$ and $x \in S$. 
\end{lemma}
\begin{proof}
To derive the form of $W_t^{\pi,\theta}$, the first step is to use $P_x^\pi$ \eqref{pxpi} to derive the induced probability measure $P_{X_t}^\pi(B) := P_x^\pi\big(\{X_t \in B \} \big)$, where $B \in \mathcal{B}_{S}$. The second step is to apply the definition of conditional expectation \cite[Thm. 6.3.3, p. 245]{ash1972}. It follows that the function $W_t^{\pi,\theta} : S \rightarrow \mathbb{R}^*$ is Borel-measurable and $W_t^{\pi,\theta}(x_t)$ is given by
%\begin{subequations}\label{85}
\begin{equation}\label{85}\begin{aligned}
  & W_t^{\pi,\theta}(x_t) \\
&    =   \textstyle \int_A \int_{S} \int_A \cdots \int_{A} \int_{S} e^{\frac{-\theta}{2} (c_N(x_N) + \sum_{i=t}^{N-1} c_i(x_i,u_i))}\\ 
  & \hphantom{=} \;\; q_{N-1}(\mathrm{d}x_{N}|x_{N-1},u_{N-1}) \; \delta_{\mu_{N-1}(x_{N-1})}(\mathrm{d}u_{N-1})  \cdots \\ & \hphantom{=} \;\; \delta_{\mu_{t+1}(x_{t+1})}(\mathrm{d}u_{t+1}) \; q_{t}(\mathrm{d}x_{t+1}|x_t,u_t) \; \delta_{\mu_t(x_t)}(\mathrm{d}u_t) \end{aligned}
\end{equation}
for all $x_t \in S$ and $t \in \mathbb{T}$.
Similarly, $W_N^{\pi,\theta} : S \rightarrow \mathbb{R}^*$ is Borel-measurable and satisfies
%\begin{equation}\label{85b}\begin{aligned}
     $W_N^{\pi,\theta}(x_N) & = e^{\frac{-\theta}{2} c_N(x_N)}$ for all $x_N \in S$.    
%\end{aligned}\end{equation}
%\end{subequations}
Since $c_t$ is bounded, we have that $W_t^{\pi,\theta}(x_t) \in (0,+\infty)$ for all $x_t \in S$ and $t \in \mathbb{T}_N$. Details about applying \cite[Thm. 6.3.3]{ash1972} are provided in a footnote.\footnote{To apply \cite[Thm. 6.3.3]{ash1972}, note that $e^{\frac{-\theta}{2} Z_t}$ is a random variable on $(\Omega,\mathcal{B}_{\Omega},P_x^\pi)$ for any $x \in S$ and $\pi \in \Pi$. $X_t$ is a random object. I.e., $X_t : \Omega \rightarrow S$ is measurable relative to $\mathcal{B}_{\Omega}$ and $\mathcal{B}_{S}$. The expectation $E_x^\pi(e^{\frac{-\theta}{2} Z_t}) := \int_{\Omega} e^{\frac{-\theta}{2} Z_t(\omega)} \mathrm{d}P_x^\pi(\omega)$ exists (is not of the form $+\infty -\infty$) because $e^{\frac{-\theta}{2} Z_t(\omega)} \geq 0$ for all $\omega \in \Omega$. While $X_t$ is a Borel-measurable function on $\Omega$ in general, our setting ensures the coordinates of $\omega \in \Omega$ are related casually.} %additional casual structure. In particular, the dynamics \eqref{dynamics} and the policy class $\Pi$ ensure that the coordinates of $\omega \in \Omega$ are related casually.}

%Let $\omega = (x_0,u_0,\dots,x_{N-1},u_{N-1},x_N) \in \Omega$. Since $e^{a+b} = e^a e^b$ for any $a \in \mathbb{R}$ and $b \in \mathbb{R}$ and $Z_t(\omega) = c_N(x_N) + \sum_{i=t}^{N-1} c_i(x_i,u_i) = c_t(x_t,u_t) + Z_{t+1}(\omega)$, it holds that
Let $t \in \{0,1,\dots,N-2\}$. By the definition of $Z_t(\omega)$ \eqref{myZt}, it holds that 
%$e^{\frac{-\theta}{2} Z_t(\omega)} = e^{\frac{-\theta}{2}c_t(x_t,u_t)}e^{\frac{-\theta}{2} Z_{t+1}(\omega)}$
%\begin{equation}\label{86}\begin{aligned}
     $e^{\frac{-\theta}{2} Z_t(\omega)} 
     %= e^{\frac{-\theta}{2} (c_t(x_t,u_t) + Z_{t+1}(\omega))}
    = e^{\frac{-\theta}{2}c_t(x_t,u_t)}e^{\frac{-\theta}{2} Z_{t+1}(\omega)}$,
%\end{aligned}\end{equation}
which equals $e^{\frac{-\theta}{2} (c_N(x_N) + \sum_{i=t}^{N-1} c_i(x_i,u_i))}$ in \eqref{85}. Since $e^{\frac{-\theta}{2}c(x_t,u_t)}$ does not depend on the trajectory after time $t$, it can be placed ``outside'' several integrals so that \eqref{85} becomes
%
%Equations \eqref{85} and \eqref{86} are used to derive the recursion \eqref{recursiondynprog}. Let $x_t \in S$. First, we provide the steps for any $t \in \{0,1,\dots,N-2\}$. By substituting \eqref{86} into \eqref{85a}, we have
%\begin{equation}\begin{aligned}
 %  & W_t^{\pi,\theta}(x_t) \\
%&    =   \textstyle \int_A \int_{S} \int_A \cdots \int_{A} \int_{S} e^{\frac{-\theta}{2}c_t(x_t,u_t)}e^{\frac{-\theta}{2} Z_{t+1}(\omega)}\\ 
 % & \hphantom{=} \; q_{N-1}(\mathrm{d}x_{N}|x_{N-1},u_{N-1}) \; \delta_{\mu_{N-1}(x_{N-1})}(\mathrm{d}u_{N-1})  \cdots \\ & \hphantom{=} \; \delta_{\mu_{t+1}(x_{t+1})}(\mathrm{d}u_{t+1}) \; q_{t}(\mathrm{d}x_{t+1}|x_t,u_t) \; \delta_{\mu_{t}(x_{t})}(\mathrm{d}u_{t}).
 % \end{aligned}\end{equation}
%Since $e^{\frac{-\theta}{2}c(x_t,u_t)}$ does not depend on the trajectory after time $t$, it can be placed ``outside'' several of the integrals as follows:
 \begin{equation}\label{89}\begin{aligned} 
    & W_t^{\pi,\theta}(x_t) \\
&    =   \textstyle \int_A e^{\frac{-\theta}{2}c_t(x_t,u_t)} \int_{S} \int_A \cdots \int_{A} \int_{S} e^{\frac{-\theta}{2} Z_{t+1}(\omega)}\\ 
  & \hphantom{=} \; q_{N-1}(\mathrm{d}x_{N}|x_{N-1},u_{N-1}) \; \delta_{\mu_{N-1}(x_{N-1})}(\mathrm{d}u_{N-1})  \cdots \\ & \hphantom{=} \; \delta_{\mu_{t+1}(x_{t+1})}(\mathrm{d}u_{t+1}) \; q_{t}(\mathrm{d}x_{t+1}|x_t,u_t) \; \delta_{\mu_{t}(x_{t})}(\mathrm{d}u_{t}).
\end{aligned}
\end{equation}
Since $t+1 \in \mathbb{T}$, by \eqref{85}, it holds that
\begin{equation}\label{90}\begin{aligned}
   W_{t+1}^{\pi,\theta}(x_{t+1})  = & \textstyle  \int_A \cdots \int_{A} \int_{S} e^{\frac{-\theta}{2} (c_N(x_N) + \sum_{i=t+1}^{N-1} c_i(x_i,u_i))}\\ 
  & q_{N-1}(\mathrm{d}x_{N}|x_{N-1},u_{N-1})  \delta_{\mu_{N-1}(x_{N-1})} (\mathrm{d}u_{N-1}) \\ &\cdots \delta_{\mu_{t+1}(x_{t+1})} (\mathrm{d}u_{t+1})
\end{aligned}\end{equation}
for all $x_{t+1} \in S$, where $e^{\frac{-\theta}{2} (c_N(x_N) + \sum_{i=t+1}^{N-1} c_i(x_i,u_i))}$ in \eqref{90} equals $e^{\frac{-\theta}{2} Z_{t+1}(\omega)}$ in \eqref{89} by applying the definition \eqref{myZt}. Moreover, the expression for $W_{t+1}^{\pi,\theta}(x_{t+1})$ \eqref{90} appears in \eqref{89}, which permits the following conclusion:
%
%Now, recall that $Z_{t+1}(\omega)$ equals $c_N(x_N) + \sum_{i=t+1}^{N-1} c_t(x_i,u_i)$ for any $\omega = (x_0,u_0,\dots,x_{N-1},u_{N-1},x_N) \in \Omega$ by \eqref{myZt}. Thus, we may substitute \eqref{90} into \eqref{89} to find that
\begin{equation}\label{114}\begin{aligned}
 & W_t^{\pi,\theta}(x_t)   = \\ & \textstyle  \int_A\hspace{-.5mm} e^{\frac{-\theta}{2}c_t(x_t,u_t)} \hspace{-.8mm}
  \int_{S} \hspace{-.5mm} W_{t+1}^{\pi,\theta}(x_{t+1})  q_{t}(\mathrm{d}x_{t+1}|x_t,u_t)  \delta_{\mu_t(x_t)}(\mathrm{d}u_t).
\end{aligned}\end{equation}
By using the definition of the Dirac measure $\delta_{\mu_{t}(x_{t})}$ and the definition of $q_t$ \eqref{qt}, we complete the derivation of the recursion for $t \in \{0,1,\dots,N-2\}$. The derivation for $t = N-1$ is analogous.
\end{proof}

The last result proves optimality.
\begin{theorem}[Optimality of $V_{0}^\theta$ and $\pi_\theta^*$]\label{optimality}
%Let $\theta \in \Theta\subseteq (-\infty,0)$. Recall that $V_{t}^\theta$ is defined by Algorithm \ref{valalgwhittle} for all $t \in \mathbb{T}_N$, $V_\theta^*$ is defined by \eqref{vthetastar}, and $\pi_\theta^*:= (\mu_{0}^\theta, \mu_{1}^\theta, \dots, \mu_{N-1}^\theta)$ satisfies \eqref{existinf}. 
Under Assumption \ref{measselect}, the equality \eqref{opteq} holds, i.e., %which we repeat below for convenience:
%\begin{equation*}
    $V_{0}^\theta(x) =  V_\theta^*(x) = \textstyle\frac{-2}{\theta}\log E_x^{\pi_\theta^*}\big(e^{\frac{-\theta}{2} Z}\big)$ for all $x \in S$.
%\end{equation*}
\end{theorem}
\begin{proof}
%Moreover, one can show that $W_t^{\pi,\theta}(x_t)\in (0,+\infty)$ for all $x_t \in S$, and the following recursion holds:
%\begin{equation}\label{recursiondynprog}\begin{aligned}
%W_t^{\pi,\theta}(x_t) = \;
%&  e^{\frac{-\theta}{2}c_t(x_t,\mu_t(x_t))} \\ & \textstyle \int_{\mathbb{R}^d} W_{t+1}^{\pi,\theta}(f_t(x_t,\mu_t(x_t),w_t)) p_t(\mathrm{d}w_t|x_t,\mu_t(x_t))
%\end{aligned}\end{equation}
%for all $t \in \mathbb{T}$ and $x_t \in S$ (see Lemma \ref{dynprogremark}, which follows %this proof).
%In addition, 
First, note that
%\begin{equation}\label{83}
     $W_0^{\pi,\theta}(x)  = E_x^\pi(e^{\frac{-\theta}{2} Z})$ for all $ x \in S$ and $\pi \in \Pi$,
%\end{equation}
and recall that $Z = Z_0$. To show the desired statement \eqref{opteq}, it suffices to show that
\begin{equation}\label{toshow84}
  \textstyle \frac{-2}{\theta} \log W_t^{\pi,\theta}(x) \geq V_{t}^\theta(x) = \frac{-2}{\theta} \log W_t^{\pi_\theta^*,\theta}(x)
\end{equation}
for all $t \in \mathbb{T}_N$, $x \in S$, and $\pi \in \Pi$. (Let $t = 0$, note that $\pi_\theta^* \in \Pi$, and use the definition of the infimum.) 
Proceed by induction. For the base case, we have
%\begin{equation}\label{my90}\begin{aligned}
   $ \frac{-2}{\theta} \log W_N^{\pi,\theta}(x)  = \frac{-2}{\theta} \log \big(e^{\frac{-\theta}{2} c_N(x)}\big)
   =  V_{N}^\theta(x)$
%\end{aligned}\end{equation}
for all $x \in S$ and $\pi \in \Pi$ because $W_N^{\pi,\theta}(x) =e^{\frac{-\theta}{2} c_N(x)}$ and by the definition of $V_{N}^\theta$. %Therefore,
%\begin{equation}
%    \textstyle  \frac{-2}{\theta} \log W_N^{\pi,\theta}(x_N) \geq V_{N}^\theta(x_N) = \textstyle  \frac{-2}{\theta} \log W_N^{\pi_\theta^*,\theta}(x_N)
%\end{equation}
%for all $x_N \in S$ and $\pi \in \Pi$, which proves the base case. 
Now, assume (the induction hypothesis) that for some $t \in \mathbb{T}$, it holds that
%\begin{equation}
$\textstyle \frac{-2}{\theta} \log W_{t+1}^{\pi,\theta}(x) \geq V_{t+1}^\theta(x) = \frac{-2}{\theta} \log W_{t+1}^{\pi_\theta^*,\theta}(x)$
%\end{equation}
for all $x \in S$ and $\pi \in \Pi$. 
%To complete the proof, we will use the induction hypothesis to show that
%\begin{equation}\label{inductionstep}
 %  \textstyle \frac{-2}{\theta} \log W_{t}^{\pi,\theta}(x_t) \geq V_{t}^\theta(x_t) = \frac{-2}{\theta} \log W_{t}^{\pi_\theta^*,\theta}(x_t)
%\end{equation}
%for all $x_t \in S$ and $\pi \in \Pi$. 
%For this, let $x_t \in S$ and $\pi = (\mu_0,\mu_1,\dots,\mu_{N-1}) \in \Pi$ be given. 
Since $\frac{-\theta}{2} > 0$, the exponential is increasing, and $e^{\log a} = a$ for all $a \in (0,+\infty)$, the induction hypothesis is equivalent to
\begin{align}
     \textstyle W_{t+1}^{\pi,\theta}(x) & \geq e^{\frac{-\theta}{2} V_{t+1}^\theta(x)} = W_{t+1}^{\pi_\theta^*,\theta}(x) \;\;\; \forall x \in S.\label{94c}
\end{align}

Now, let $x \in S$ and $\pi = (\mu_0,\mu_1,\dots,\mu_{N-1}) \in \Pi$ be given. We use the recursion provided by Lemma \ref{dynprogremark}, the inequality in \eqref{94c}, $V_{t+1}^\theta$ being lsc and bounded below (Thm. \ref{lscremark}), and $W_{t+1}^{\pi,\theta}$ being Borel-measurable 
%, and $e^{\frac{-\theta}{2}c_t(x,\mu_t(x))} \in (0,+\infty)$ 
to conclude that
\begin{equation}\label{mymy46}\begin{aligned}
& W_t^{\pi,\theta}(x)
 \geq \\ & \textstyle e^{\frac{-\theta}{2}c_t(x,\mu_t(x))}   \int_{\mathbb{R}^d} e^{\frac{-\theta}{2} V_{t+1}^\theta(f_t(x,\mu_t(x),w))} \; p_t(\mathrm{d}w|x,\mu_t(x)).
\end{aligned}\end{equation}
%by applying \cite[Thm. 1.5.9 (b), p. 41]{ash1972}.
The right-hand-side of the inequality in \eqref{mymy46} is a product of elements of $(0,+\infty)$ in particular since $V_{t+1}^\theta$ is bounded (Thm. \ref{lscremark}). Since $\log(a b) = \log a + \log b$ for any $a \in (0,+\infty)$ and $b \in (0,+\infty)$, the natural logarithm is increasing, and $W_t^{\pi,\theta}(x) \in (0,+\infty)$, it holds that
\begin{equation}\begin{aligned}
    &  \log W_t^{\pi,\theta}(x) \\
    & \geq  \textstyle \log e^{\frac{-\theta}{2}c_t(x,\mu_t(x))} \\ & \hphantom{\geq} \; + \textstyle \log \int_{\mathbb{R}^d} e^{\frac{-\theta}{2} V_{t+1}^\theta(f_t(x,\mu_t(x),w))}  p_t(\mathrm{d}w|x,\mu_t(x)).
\end{aligned}\end{equation}
By simplifying the first term in the sum and multiplying by $\frac{-2}{\theta}> 0$, it follows that $\frac{-2}{\theta} \log W_t^{\pi,\theta}(x) \geq v_{t+1}^\theta(x,\mu_t(x))$, where $v_{t+1}^\theta$ is given by \eqref{mypsi}.
%\begin{equation}\begin{aligned}
 %   & \textstyle \frac{-2}{\theta} \log W_t^{\pi,\theta}(x_t) \\
 %   & \geq  \textstyle c_t(x_t,\mu_t(x_t)) \\ & \hphantom{\geq} \; + \textstyle \frac{-2}{\theta} \log \int_{\mathbb{R}^d} e^{\frac{-\theta}{2} V_{t+1}^\theta(f_t(x_t,\mu_t(x_t),w_t))}  p_t(\mathrm{d}w_t|x_t,\mu_t(x_t))\\
 %   & = v_{t+1}^\theta(x_t,\mu_t(x_t)),
%\end{aligned}\end{equation}
%where we used the definition of $v_{t+1}^\theta$ \eqref{10c} to write the last line.
Since $v_{t+1}^\theta(x,\mu_t(x)) \geq \inf_{u \in A}v_{t+1}^\theta(x,u) = V_t^\theta(x)$ \eqref{10b}, we conclude that $\frac{-2}{\theta} \log W_t^{\pi,\theta}(x) \geq V_{t}^\theta(x)$.
%\begin{equation}
 %    {\textstyle \frac{-2}{\theta}} \log W_t^{\pi,\theta}(x_t)
    %\geq \inf_{u_t \in A} v_{t+1}^\theta(x_t,u_t) = V_{t}^\theta(x_t),
%\end{equation}
%where we used the definition of $V_{t}^\theta$ \eqref{10b} to write the equality. 

A similar procedure shows that $V_{t}^\theta(x) = \frac{-2}{\theta} \log W_{t}^{\pi_\theta^*,\theta}(x)$ to complete the induction. In particular, one uses $\pi = \pi_\theta^* := (\mu_{0}^\theta, \mu_{1}^\theta, \dots, \mu_{N-1}^\theta) \in \Pi$ in the recursion provided by Lemma \ref{dynprogremark}, where each $\mu_{t}^\theta : S \rightarrow A$ is Borel-measurable and satisfies \eqref{existinf}. Such a function exists by Theorem \ref{lscremark}.
\end{proof}
